# Supplementary material for: Optical bound states in the continuum in subwavelength gratings made of an epitaxial van der Waals material
Source: arXiv:2502.03121 source file (2025-02-05)
Supplement: Supplementary file 1 [file suppinf2.pdf]

# Supporting Information to "Optical bound states in the continuum in subwavelength gratings made of an epitaxial van der Waals material"

Emilia Pruszyńska-Karbownik,[1] Tomasz Fąs,[1] Katarzyna Brańko,[1] Dmitriy Yavorskiy,[2,3,4] Bartłomiej Stonio,[5] Rafał Bożek,[1] Piotr Karbownik,[6] Jerzy Wróbel,[3] Tomasz Czyszanowski,[7] Tomasz Stefaniuk,[1] Wojciech Pacuski,[1] and Jan Suffczyński[1]

[1] *Faculty of Physics, University of Warsaw, Pasteura St. 5, 02-093 Warsaw, Poland**
[2] *Institute of High Pressure Physics Polish Academy of Sciences, 29/37 Sokolowska St., 01-142 Warsaw, Poland*
[3] *Institute of Physics, Polish Academy of Sciences, 32/46 Lotnikow Av., 02-668 Warsaw, Poland*
[4] *CENTERA, CEZAMAT, Warsaw University of Technology, 19 Poleczki Str., 02-822 Warsaw, Poland*
[5] *CEZAMAT, Warsaw University of Technology, Poleczki 19, 02-822, Warsaw, Poland*
[6] *Center of Development and Implementation, Telesystem-Mesko Sp. z o.o, ul. Warszawska 51, 05-082, Lubiczów, Poland*
[7] *Institute of Physics, Łódź University of Technology, 217/221 Wólczańska St., 90-451 Łódź, Poland*

(Dated: January 14, 2025)

This file contains supporting information to the article "Optical bound states in the continuum in subwavelength gratings made of an epitaxial van der Waals materia".

## REFRACTIVE INDEX OF THE SAPPHIRE SUBSTRATE

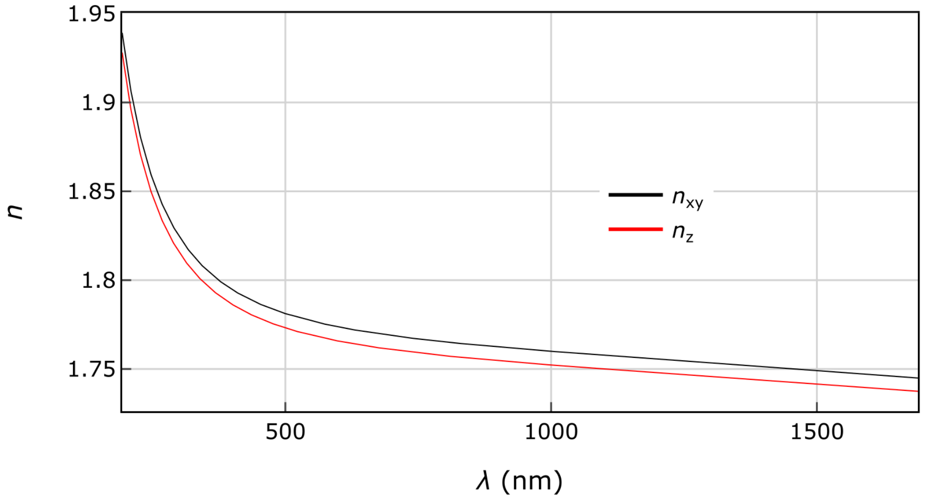


Figure S1: Real part of in-plane $n_{xy}$ and out-of-plane refractive index $n_z$ of the (0001) $Al_2O_3$ substrate with a 2-degree off-cut determined by ellipsometry measurements. The imaginary parts of the refractive index are zero in the both cases.

* emilia.karbownik@fuw.edu.pl

## DESIGN OF THE $MoSe_2$-BASED SUBWAVELENGTH GRATINGS BY THEORETICAL CALCULATIONS

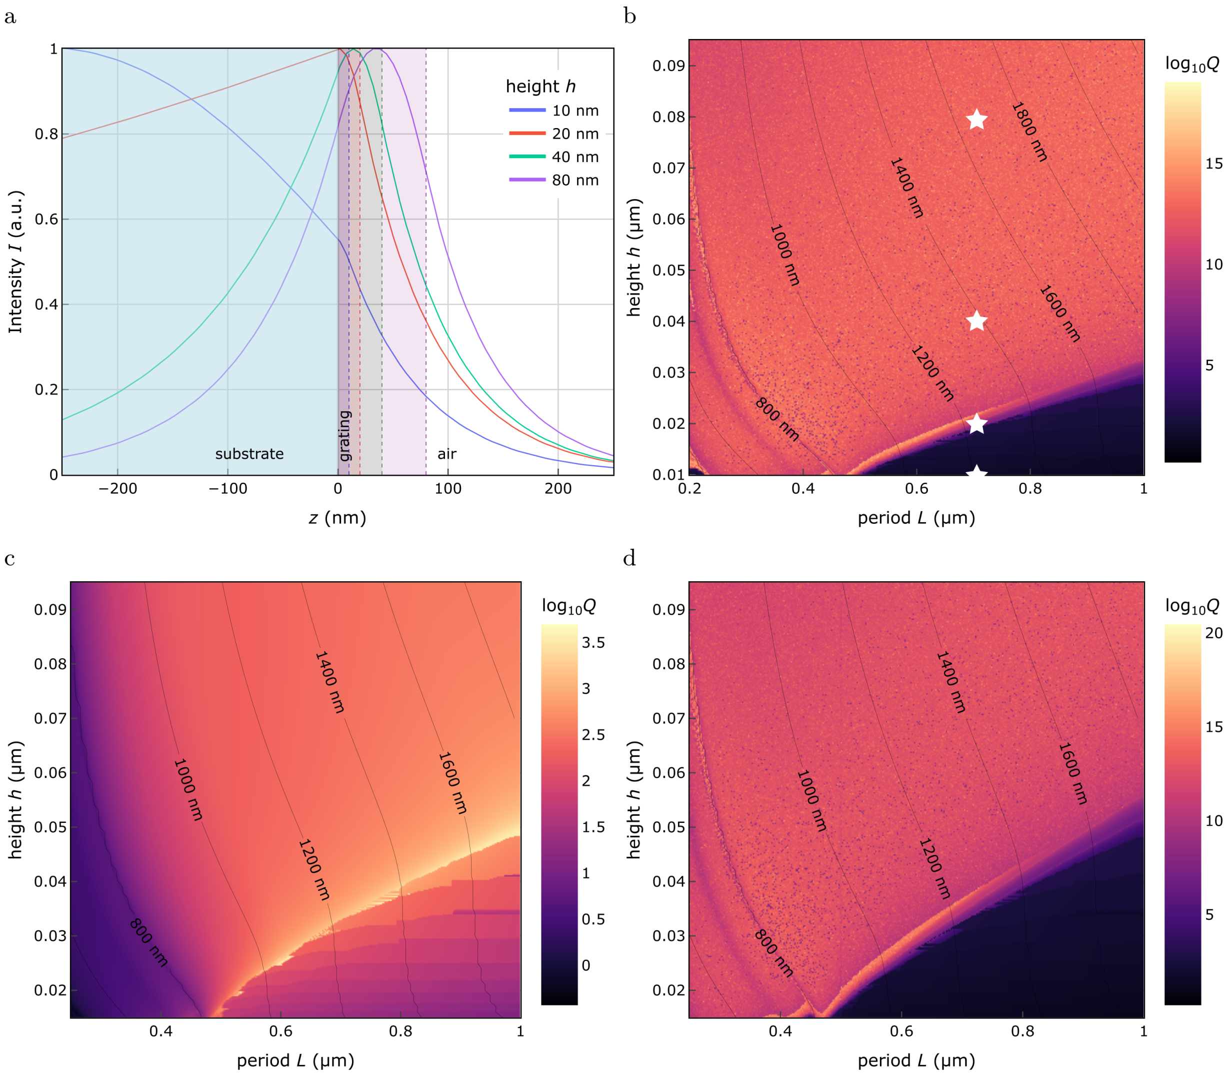


Figure S2: a) Numerically calculated light intensity distributions of the mode $TE_{10}$ in $z$ direction in the structure with period $L = 700$nm, fill factor $F = 0.8$, and different height $h$ values. The colored regions indicate respective parts of the structure: the substrate and the grating, while the area above the grating is indicated in white. b) Numerically calculated maps of Q-factor of the mode $TE_{10}$ for fill-factor $F = 0.8$ with the assumption of the lack of the absorption, c) for $F = 0.5$ with absorption, d) for $F = 0.5$ without absorption. The calculated wavelengths of the mode are marked with the contour lines, white stars indicate the gratings from the a) panel.

## REFLECTIVITY AND TRANSMISSION OF THE MBE-GROWN $MoSe_2$ LAYERS

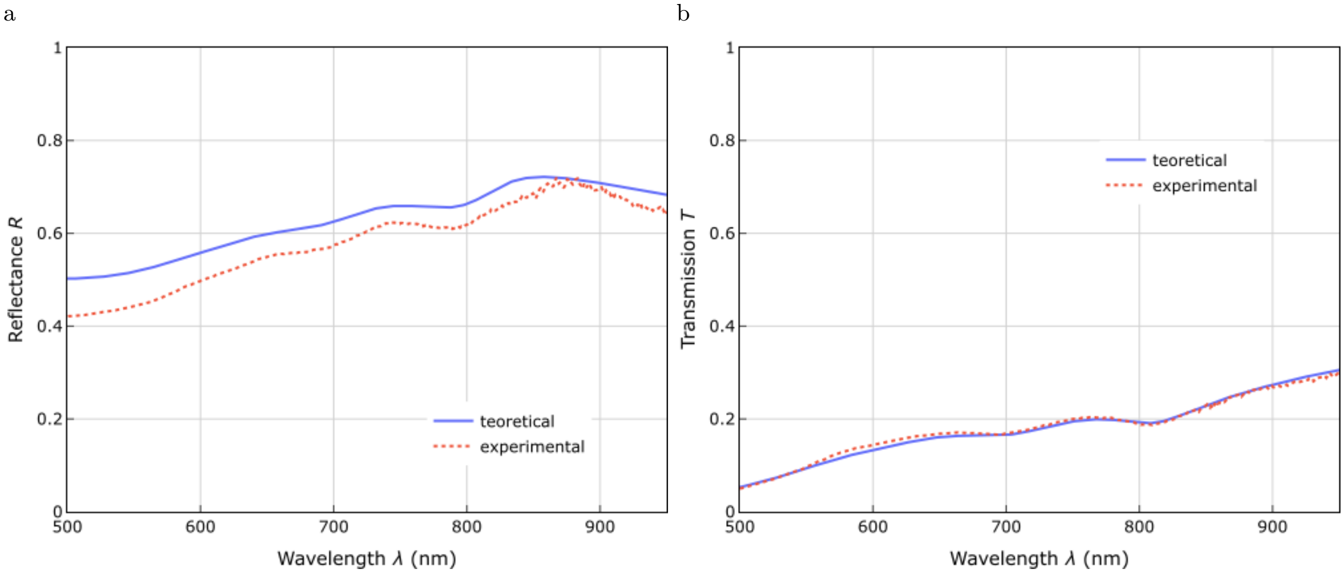


Figure S3: Experimental reflectivity (a) and transmission (b) spectra of the MBE layers measured perpendicular to the sample using a spectrometer and obtained by numerical calculations for plain 42-nm layer $MoSe_2$ laying on a sapphire substrate.

## BOUND STATE IN THE CONTINUUM IN THE PRESENCE OF A NET ABSORPTION

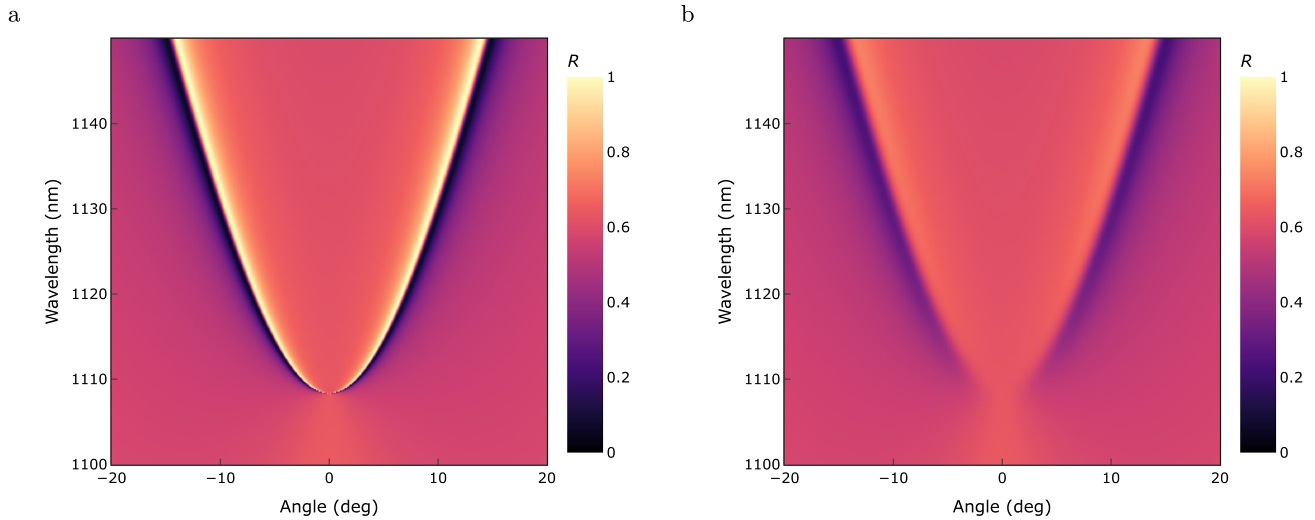


Figure S4: Numerically calculated angle-resolved reflectivity maps in the area of the dispersion curve of $TE_{10}$ mode of the $MoSe_2$-based subwavelength grating a) with the assumption of no material losses b) when taking into account the material losses as presented in Fig. 3c. The real wavelength of mode is $\lambda = 1108.4$ nm and Q-factors at zero angle are $Q_{Rz} = 1.6 \cdot 10^8$ in a) and $Q_{abs} = 206.9$ in b).

## CUT-OFFS OF THE FIRST DIFFRACTION ORDER OF A GRATING

We consider the first diffraction order of a diffraction grating with period $L$. Light incident at an angle of $\alpha$ will be diffracted at an angle $\beta$, such that

$$\sin\alpha \pm sin\beta = \frac{\lambda}{nL}, \tag{1}$$

where $\lambda$ is the wavelength of the light and $n$ – the refractive index of the surroundings. The sign depends on whether the grating is reflective or transmissive.

Because $-1 \leq \sin\beta \leq 1$ and all other variables are positive the above equation reduces to

$$\lambda \leq nL\left(\sin\alpha + 1\right), \tag{2}$$

in both cases. The cut-off lines of this condition are visible on reflectivity maps and they crosses for the wavelength equal to the period of the grating (the cut-off for the propagation in the air) and equal to the period times the refractive index of the substrate (the cut-off for the propagation in the substrate).

## 3D TOMOGRAPHY OF THE REFLECTIVITY OF THE $MoSe_2$ GRATINGS

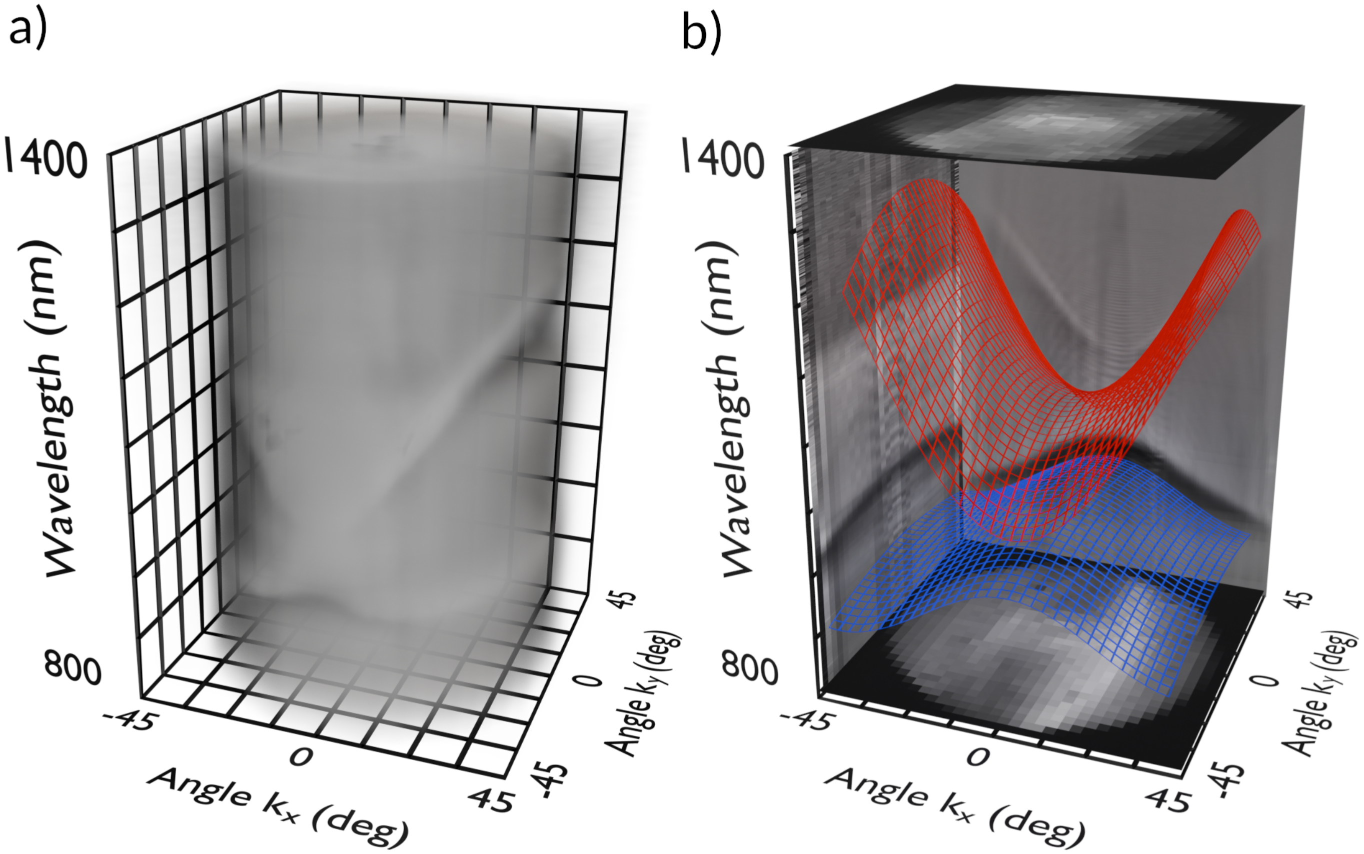


Figure S5: Energy position of the modes determined in experiment as a function of the in-plane photon momentum $k_x$ and $k_y$. Cross-sections of the volume cut along $k_x = 0$ and $k_y = 0$ planes are projected onto $k_x - k_y$ plane. Here we show $TE_{10}$ mode (top) and $TE_{20}$ (bottom). Those slices are later used for the calculation of polarization vortices. The upper branch displays a saddle-like dispersion.

Supp. Fig. S5 presents the results of 3D tomography measurements of the optical modes of the $MoSe_2$-based grating in reflectivity. The Supp. Fig. S5a shows the registered volume in the $k$-space, while Supp. Fig. S5b presents energy of the TE modes (red and blue grids) as a function of the in-plane photon momentum $k_x$ and $k_y$. The cross-sections of the k-space along $k_x$ at $k_y = 0$ and along $k_y$ at $k_x = 0$ are displayed on the vertical planes of the plot. The cross-sections of the $k$-space in the horizontal direction for $k = 0$ respectively for the lower and higher wavelength mode are displayed on the bottom and top horizontal surfaces of the plot.

## OPTICAL MICROSCOPE IMAGE OF THE SAMPLE SURFACE

An image of the sample surface acquired using an optical microscope is shown in Figure S6. An array of $MoSe_2$-based subwavelength gratings etched out of 42 nm thick layer of $MoSe_2$ is evidenced. A variation in the color of the gratings reflects the variation in the gratings geometry parameters.

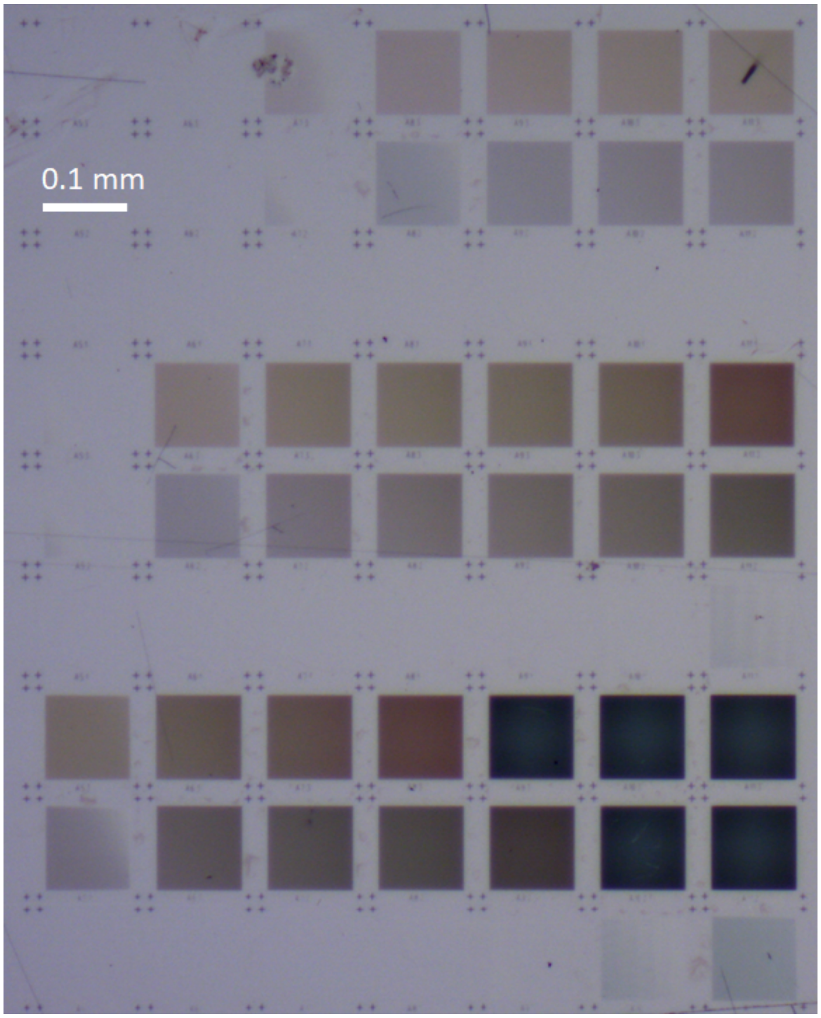


Figure S6: Optical microscope image of the sample with a set of $MoSe_2$ subwavelength gratings etched out of 42 nm thick layer of $MoSe_2$. An array of $MoSe_2$-based subwavelength gratings with 100 µm × 100 µm dimensions are evidenced.

## SCHEMES OF THE EXPERIMENTAL SETUPS

## DEPENDENCE OF THE THIRD-HARMONIC SIGNAL INTENSITY ON THE WAVELENGTH

The nonlinearity of $MoSe_2$, like that of other TMDs, is highly dependent on the thickness of the film due to the interplay of lattice symmetry, quantum confinement, and interlayer interactions [S71]. In a monolayer of $MoSe_2$, inversion symmetry is absent due to the asymmetric positioning of the selenium atoms in the top and bottom layers relative to the central molybdenum atomic layer. This lack of symmetry is essential for enabling second harmonic generation (SHG), as under the electric dipole approximation, the inversion symmetry causes the nonlinear polarization to reverse sign, canceling the second-order response. However, as additional layers are stacked, typically in an AB sequence, the atomic arrangement creates interlayer symmetry. In this configuration, the atomic arrangement within each layer compensates for the asymmetry of adjacent layers, thereby restoring the material's centrosymmetricity and suppressing nonlinear effects such as SHG. Moreover, as the thickness of $MoSe_2$ increases, the quantum confinement effect diminishes due to the delocalization of electronic wavefunctions across the additional layers. This leads to significant modifications in the band structure, causing the material to transition from a direct bandgap in the monolayer to an indirect bandgap in the bulk. Consequently, nonlinear optical processes are weakened as a result of reduced dipole transition strengths and lower optical absorption associated with the indirect bandgap configuration. Given that our $MoSe_2$ layer is 42 nm thick (approximately 60 atomic layers), the generation of second-harmonic light in this case would primarily arise from a symmetry breaking at the surface interfaces rather than within the bulk

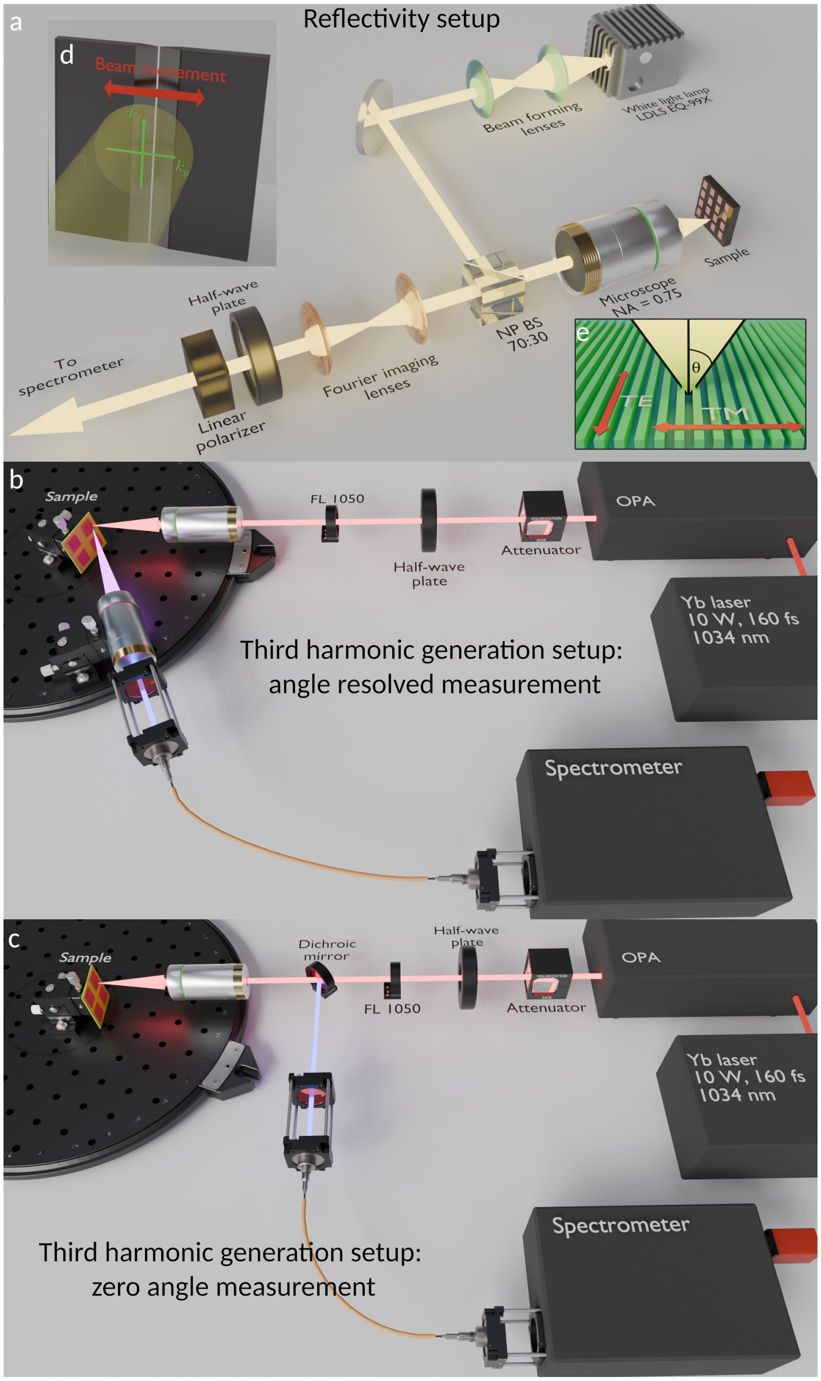


Figure S7: Schematics of the experimental setups (top) for k-space imaging, (center) for nonlinear investigations for non-zero angles, (bottom) for nonlinear investigations for the zero angle. Inset (a) presents directions of polarization and angles in the experiments, while inset (b) – the beam alignment with the spectrometer slit in the setup for k-space imaging. The schematics contain assets made by Ryo Mizuta Graphics and models from Thorlabs catalog.

volume. Furthermore, since the electric field in TE-polarized BIC is along the grating stripes, its orientation limits interaction with symmetry-breaking features, making it hard to harness the field enhancement associated with the BIC effectively. Our experiment confirms the absence of efficient second harmonic generation in our samples (not shown), in consistency with the above discussion.

The nonlinear optical response of the $MoSe_2$ layer-based subwavelength grating. The intensity of THG generated under 27-degree excitation for a) TE and b) TM polarization. c) The wavelength dependence of the enhancement

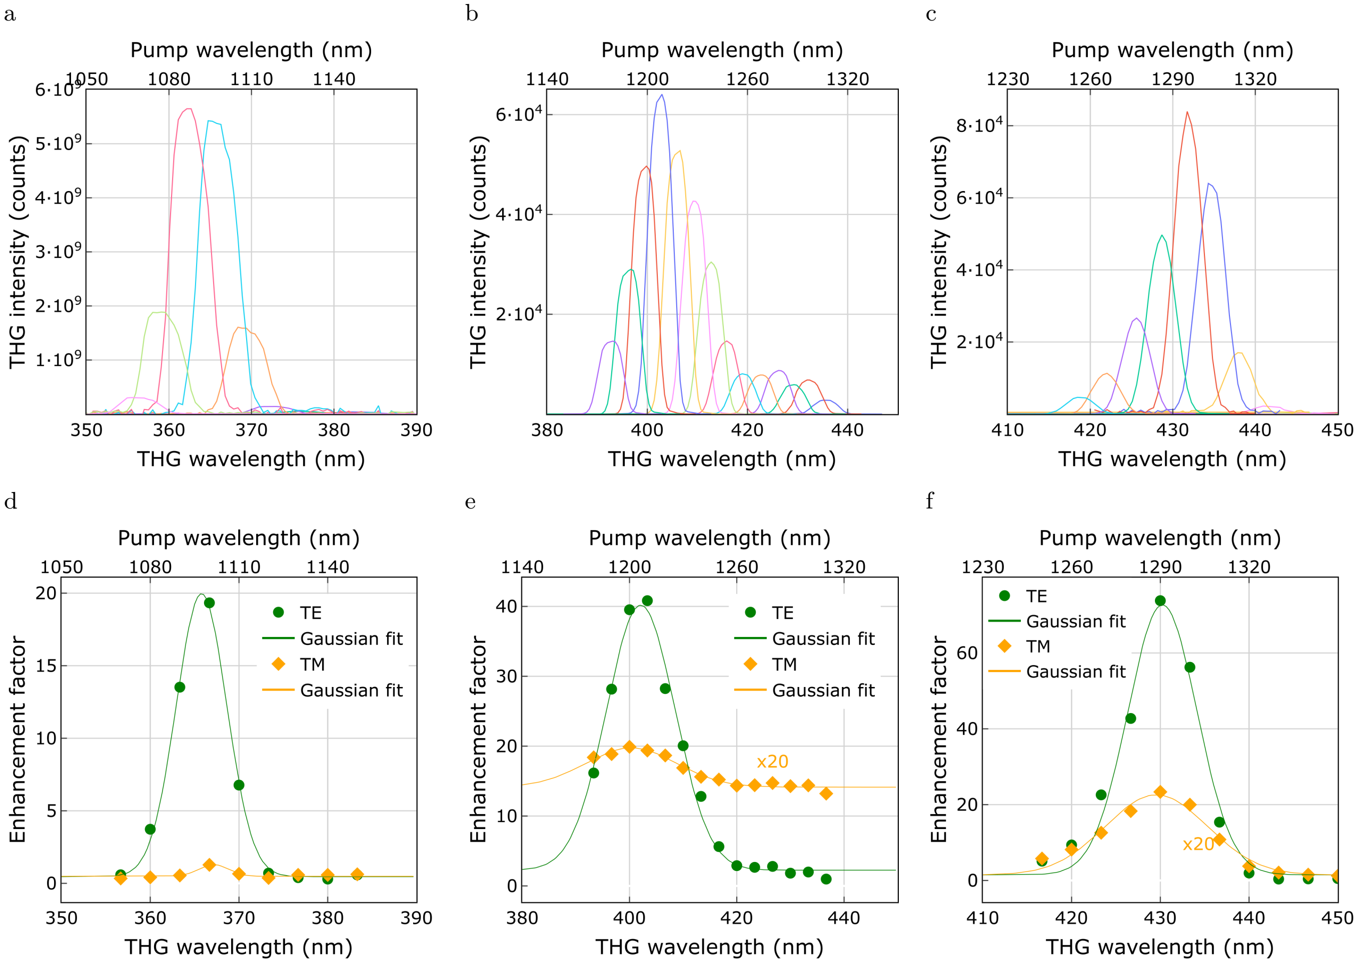


Figure S8: The nonlinear optical response of the $MoSe_2$ layer-based subwavelength grating. The intensity of THG signal generated for TE polarization under excitation under a) 0-degree b) 34-degree and c) 45-degree to normal. The wavelength dependence of the enhancement factor at d) 0-degree e) 34-degree and f) 45-degree to normal for TE and TM polarizations.

factor at a 27-degree angle for both polarizations. d) The angular dependence of the maximum observed enhancement factor is shown in Supp. Figure S8.
